# Supplementary material for: Organic-mineral interactions under natural conditions -- a computational study of flavone adsorption on smectite clay
Source: arXiv:2212.11428 source file (2022-12-22)
Supplement: Supplementary file 1 [file SI.pdf]

# Interactions of flavone apigenin and smectite clay: the effect of pH and cations on the adsorption

Omar Nuruzade,[1,2] Elshan Abdullayev,[1] and Valentina Erastova[3]*

[1] Department of Life Sciences, Khazar University, 41 Mahsati Street, Baku, AZ1096, Azerbaijan
[2] Department of Oil and Gas Engineering, French-Azerbaijani University, 183 Nizami Street, Baku, AZ1000, Azerbaijan
[3] School of Chemistry, University of Edinburgh, Joseph Black Building, David Brewster Road, King's Buildings, Edinburgh, EH9 3FJ, UK

* valentina.erastova@ed.ac.uk

## Supplementary Information

**Table S1:** Apigenin species molar fraction distribution in % across pH. The pH range of relevance to this study is highlighted, the dominant (> 15%) ranges for the apigenin species are shown in bold, while the non-dominant species (<15%) are greyed out.

| | $Api^0$ | Not used | $Api^{1-}$ | Not used | $Api^{2-}$ | Not used | Not used | $Api^{3-}$ |
|---|---|---|---|---|---|---|---|---|
| **pH** | 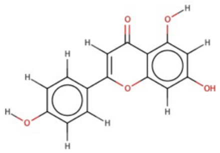 | 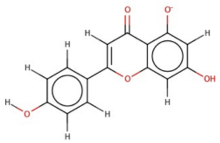 | 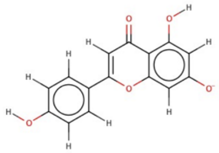 | | 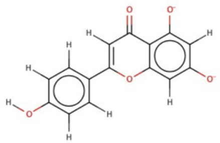 | | 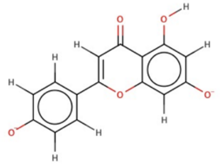 | 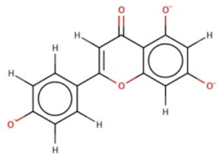 |
| **0** | 100 | 0 | 0 | 0 | 0 | 0 | 0 | 0 |
| **0.5** | 100 | 0 | 0 | 0 | 0 | 0 | 0 | 0 |
| **1** | 100 | 0 | 0 | 0 | 0 | 0 | 0 | 0 |
| **1.5** | 100 | 0 | 0 | 0 | 0 | 0 | 0 | 0 |
| **2** | 100 | 0 | 0 | 0 | 0 | 0 | 0 | 0 |
| **2.5** | 99.99 | 0 | 0.01 | 0 | 0 | 0 | 0 | 0 |
| **3** | 99.97 | 0 | 0.02 | 0 | 0 | 0 | 0 | 0 |
| **3.5** | 99.92 | 0.01 | 0.07 | 0 | 0 | 0 | 0 | 0 |
| **4** | **99.73** | 0.04 | 0.23 | 0 | 0 | 0 | 0 | 0 |
| **4.5** | **99.16** | 0.11 | 0.71 | 0.01 | 0 | 0 | 0 | 0 |
| **5** | **97.4** | 0.36 | 2.22 | 0.02 | 0 | 0 | 0 | 0 |
| **5.5** | **92.21** | 1.06 | 6.65 | 0.06 | 0.02 | 0 | 0 | 0 |
| **6** | **78.83** | 2.87 | **17.97** | 0.15 | 0.14 | 0.01 | 0.03 | 0 |
| **6.5** | **53.63** | 6.18 | **38.65** | 0.32 | 0.94 | 0.04 | 0.23 | 0.01 |
| **7** | **25.71** | 9.37 | **58.59** | 0.49 | 4.49 | 0.18 | 1.11 | 0.08 |
| **7.5** | 8.5 | 9.8 | **61.25** | 0.51 | **14.83** | 0.58 | 3.65 | 0.88 |
| **8** | 1.87 | 6.84 | **42.72** | 0.35 | **32.71** | 1.29 | 8.06 | 6.16 |
| **8.5** | 0.24 | 2.79 | **17.43** | 0.14 | **42.2** | 1.66 | 10.4 | **25.13** |
| **9** | 0.02 | 0.63 | 3.93 | 0.03 | **30.1** | 1.19 | 7.42 | **56.68** |

*cont.*

*cont.*

| | | | | | | | | |
|---|---|---|---|---|---|---|---|---|
| **9.5** | 0 | 0.09 | 0.57 | 0 | 13.72 | 0.54 | 3.38 | **81.7** |
| **10** | 0 | 0.01 | 0.06 | 0 | 4.97 | 0.2 | 1.22 | 93.54 |
| **10.5** | 0 | 0 | 0.01 | 0 | 1.64 | 0.06 | 0.41 | 97.88 |
| **11** | 0 | 0 | 0 | 0 | 0.53 | 0.02 | 0.13 | 99.32 |
| **11.5** | 0 | 0 | 0 | 0 | 0.17 | 0.01 | 0.04 | 99.78 |
| **12** | 0 | 0 | 0 | 0 | 0.05 | 0 | 0.01 | 99.93 |
| **12.5** | 0 | 0 | 0 | 0 | 0.02 | 0 | 0 | 99.98 |
| **13** | 0 | 0 | 0 | 0 | 0.01 | 0 | 0 | 99.99 |
| **13.5** | 0 | 0 | 0 | 0 | 0 | 0 | 0 | 100 |
| **14** | 0 | 0 | 0 | 0 | 0 | 0 | 0 | 100 |

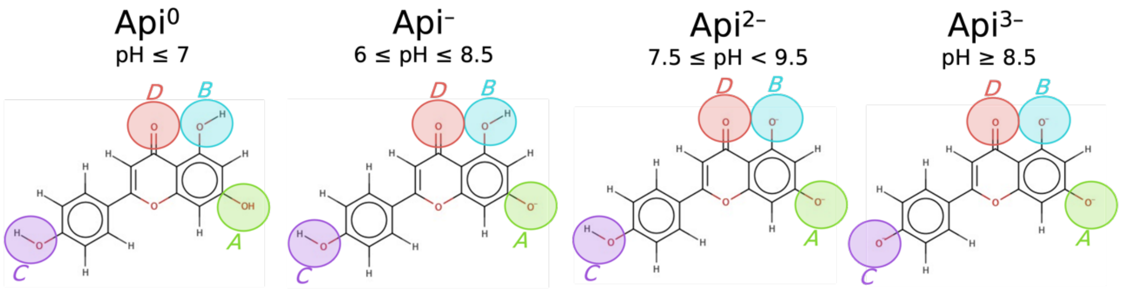


**Figure S1**: Apigenin protonation states and their dominant pH ranges, where species are present over >15% (see **Table S1**). Specie names and oxygen group names given as used in the analysis.

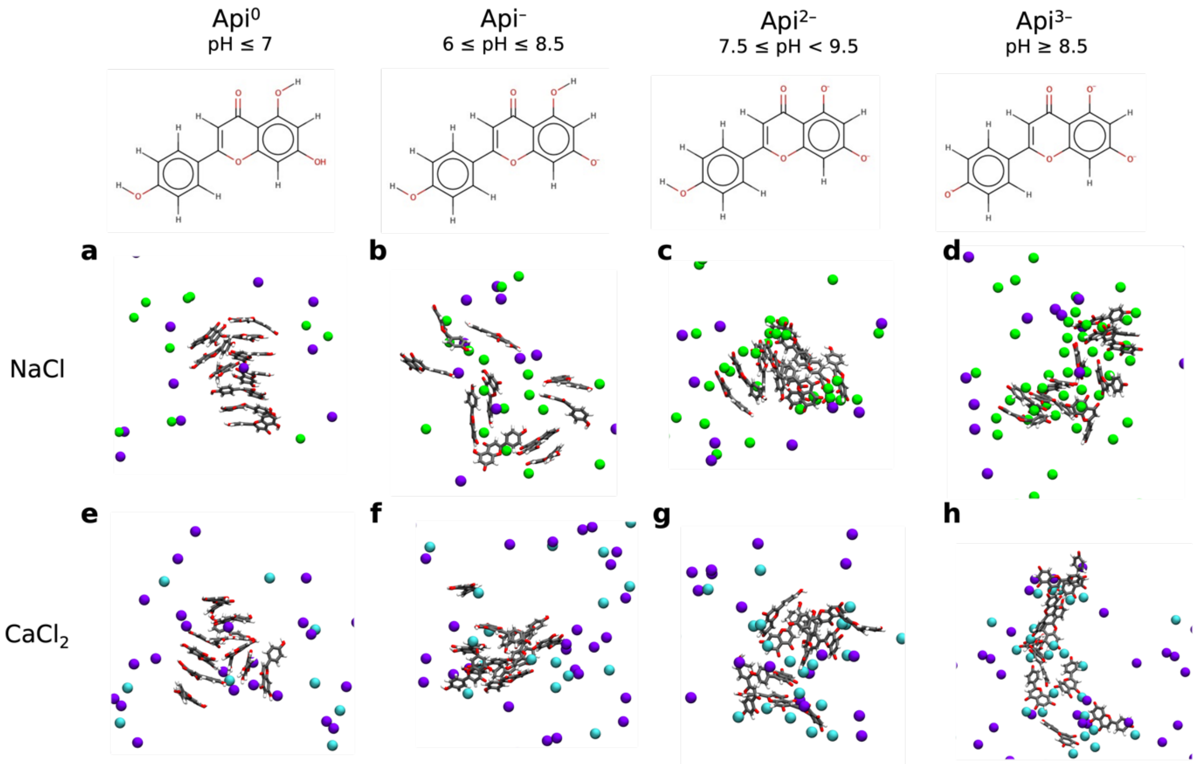


**Figure S2**: Snapshots after 50 ns simulation of apigenin systems and their pH ranges, with the specified counterbalancing ions and the 0.1M of named salt solution. Rendering with VMD, colors: Apigenin species – C grey, H white, O red; Ions – $Na^+$ green, $Ca^{2+}$ cyan, $Cl^-$ purple, water is not shown for clarity.

**Table S2**: Montmorillonite (MMT) clay unit cell composition of a model used in this study and its experimental counterpart – Wyoming montmorillonite, SWy.

| | Counter ions | Octahedral sheet | Tetrahedral sheet and OH |
|---|---|---|---|
| **Model:** | $Ca_{0.11}$ $Na_{0.343}$ | $Al_3$ $Fe^{III}_{0.43}$ $Mg_{0.57}$ | $Si_8$ $O_{20}$ $(OH)_4$ |
| **Experimental:** | $Ca_{0.12}$ $Na_{0.32}$ $K_{0.05}$ | $Al_{3.01}$ $Fe^{III}_{0.41}$ $Mg_{0.54}$ $Mn_{0.01}$ $Ti_{0.02}$ | $Si_{7.98}$ $Al_{0.02}$ $O_{20}$ $(OH)_4$ |

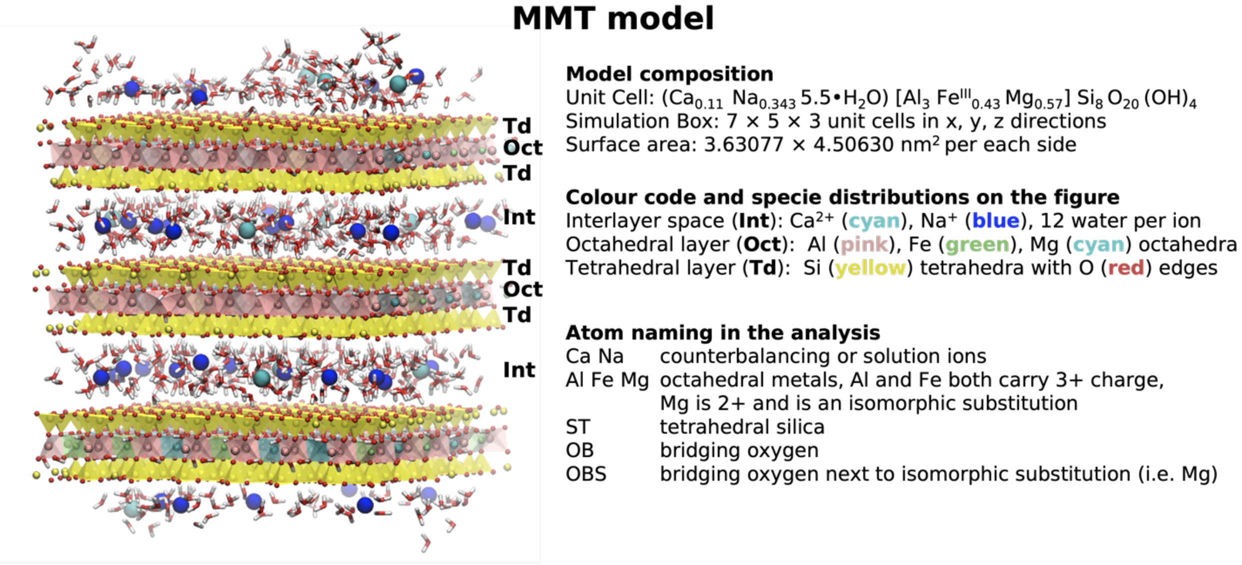


**Figure S3**: Description of the model of Wyoming montmorillonite clay (MMT), including its compassion, surface area, specie distributions and colors for the rendering, and atom naming used in the analysis.

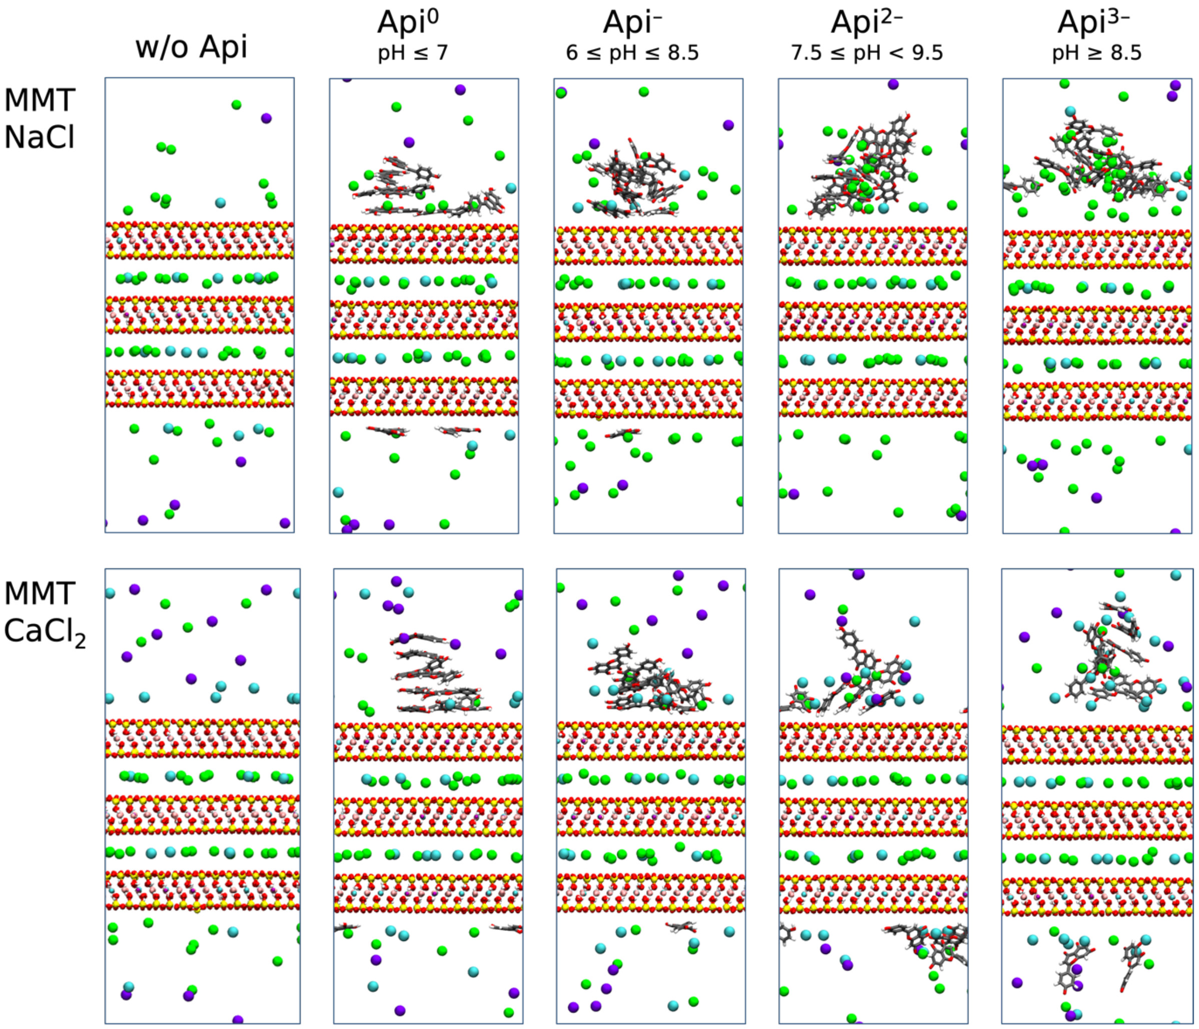


**Figure S4**: Snapshots of (left column) MMT (after 20 ns simulation) and apigenin-MMT (after 100 ns simulation) with the species at the given pH ranges, with the (Ficounterbalancing ions and the 0.1M of NaCl (top row) or $CaCl_2$ (bottom row) salt solution. Rendering with VMD, colors: Apigenin species – C grey, H white, O red; Ions – $Na^+$ green, $Ca^{2+}$ cyan, $Cl^-$ purple; Clay – Si yellow, O red, H white, Al pink, Mg cyan, Fe green, water is not shown for clarity.

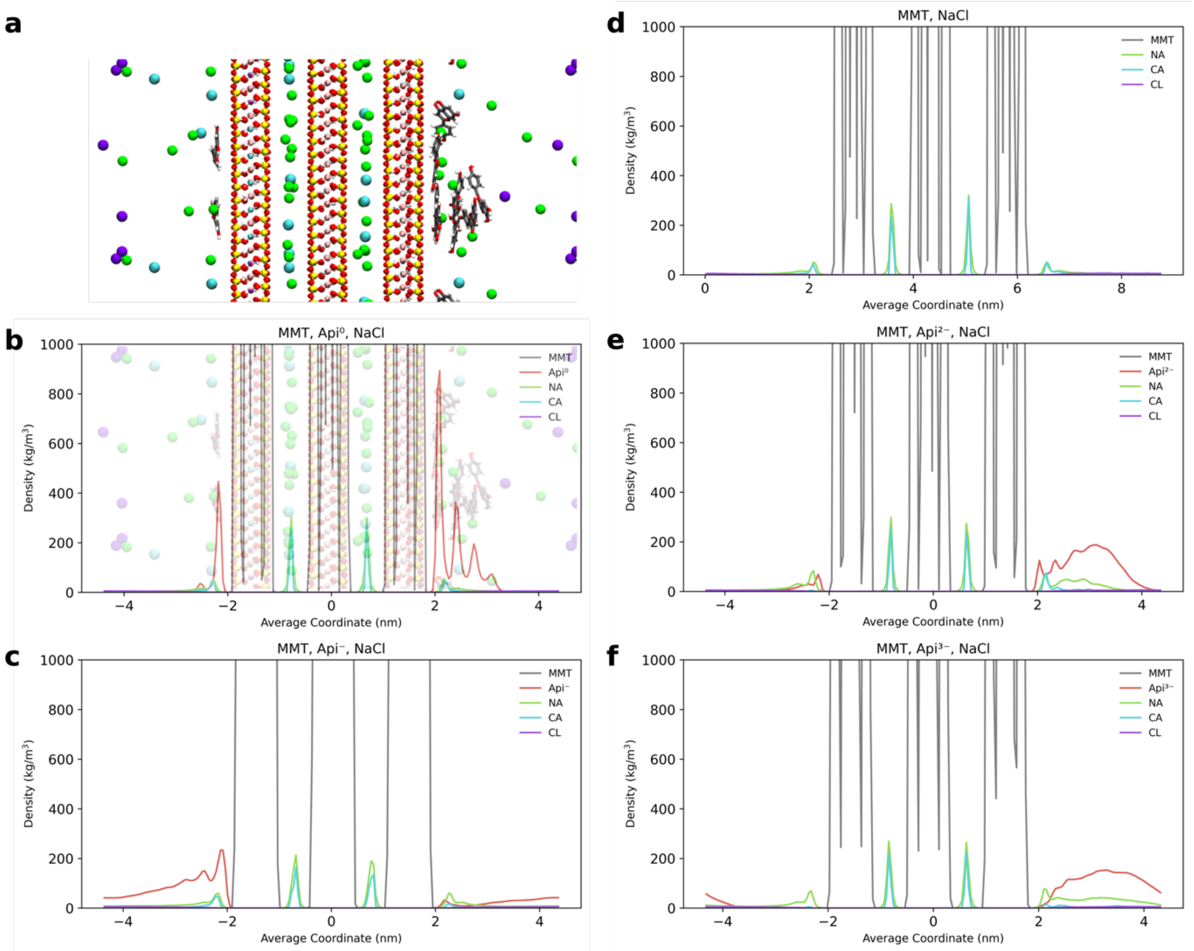


**Figure S5**: Density profiles for systems with 0.1 M NaCl solution: (**a**) rendering of a system containing $Api^0$, MMT and ions projected along z-axis; (**b**) linear density along z-axis of the system (**a**); (**c**), (**e**) and (**f**) are MMT – apigenin systems for the $Api^-$, $Api^{2-}$ and $Api^{3-}$ respectively; (**d**) is a profile for reference system without apigenin.

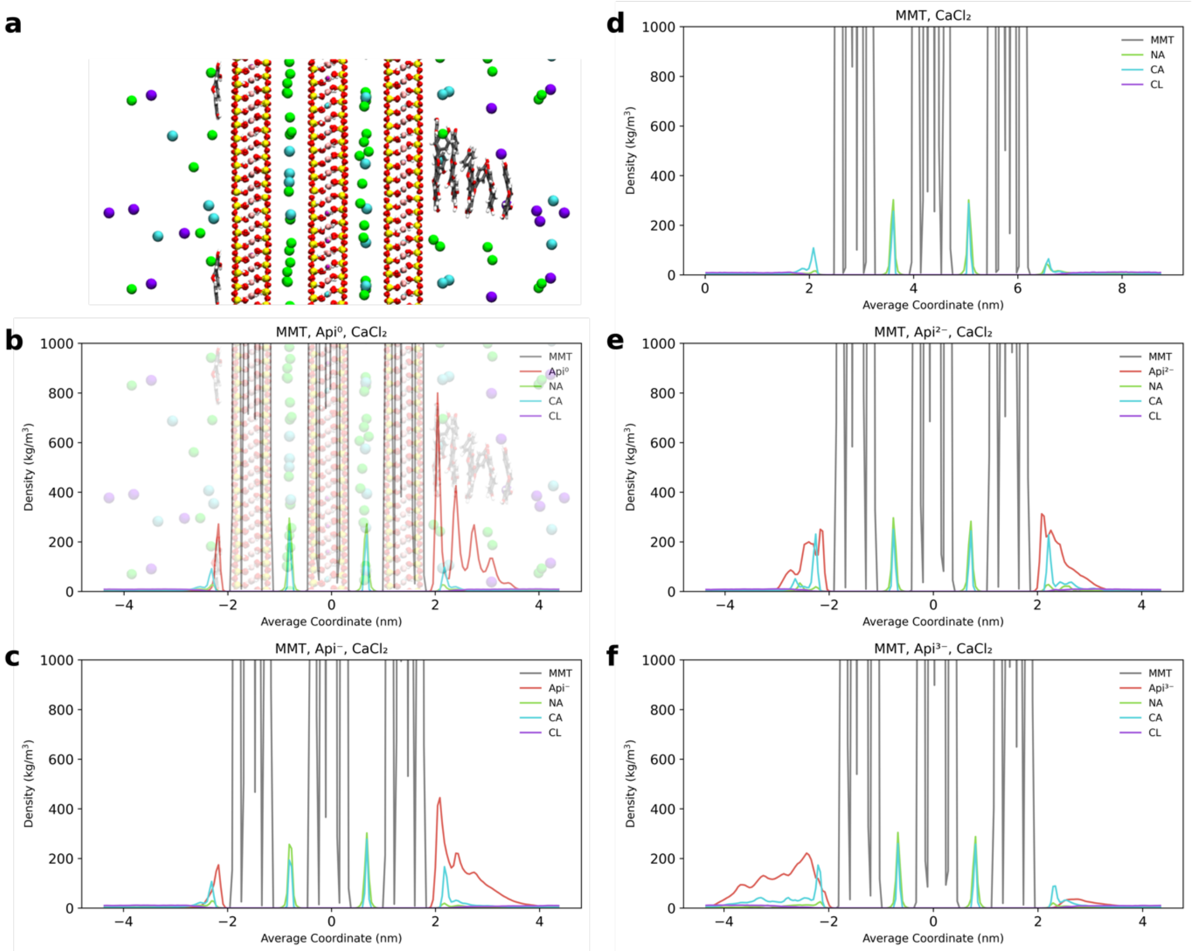


**Figure S6**: Density profiles for systems with 0.1M $CaCl_2$ solution: (**a**) rendering of a system containing $Api^0$, MMT and ions projected along z-axis; (**b**) linear density along z-axis of the system (**a**); (**c**), (**e**) and (**f**) are MMT – apigenin systems for the $Api^-$, $Api^{2-}$ and $Api^{3-}$ respectively; (**d**) is a profile for reference system without apigenin.

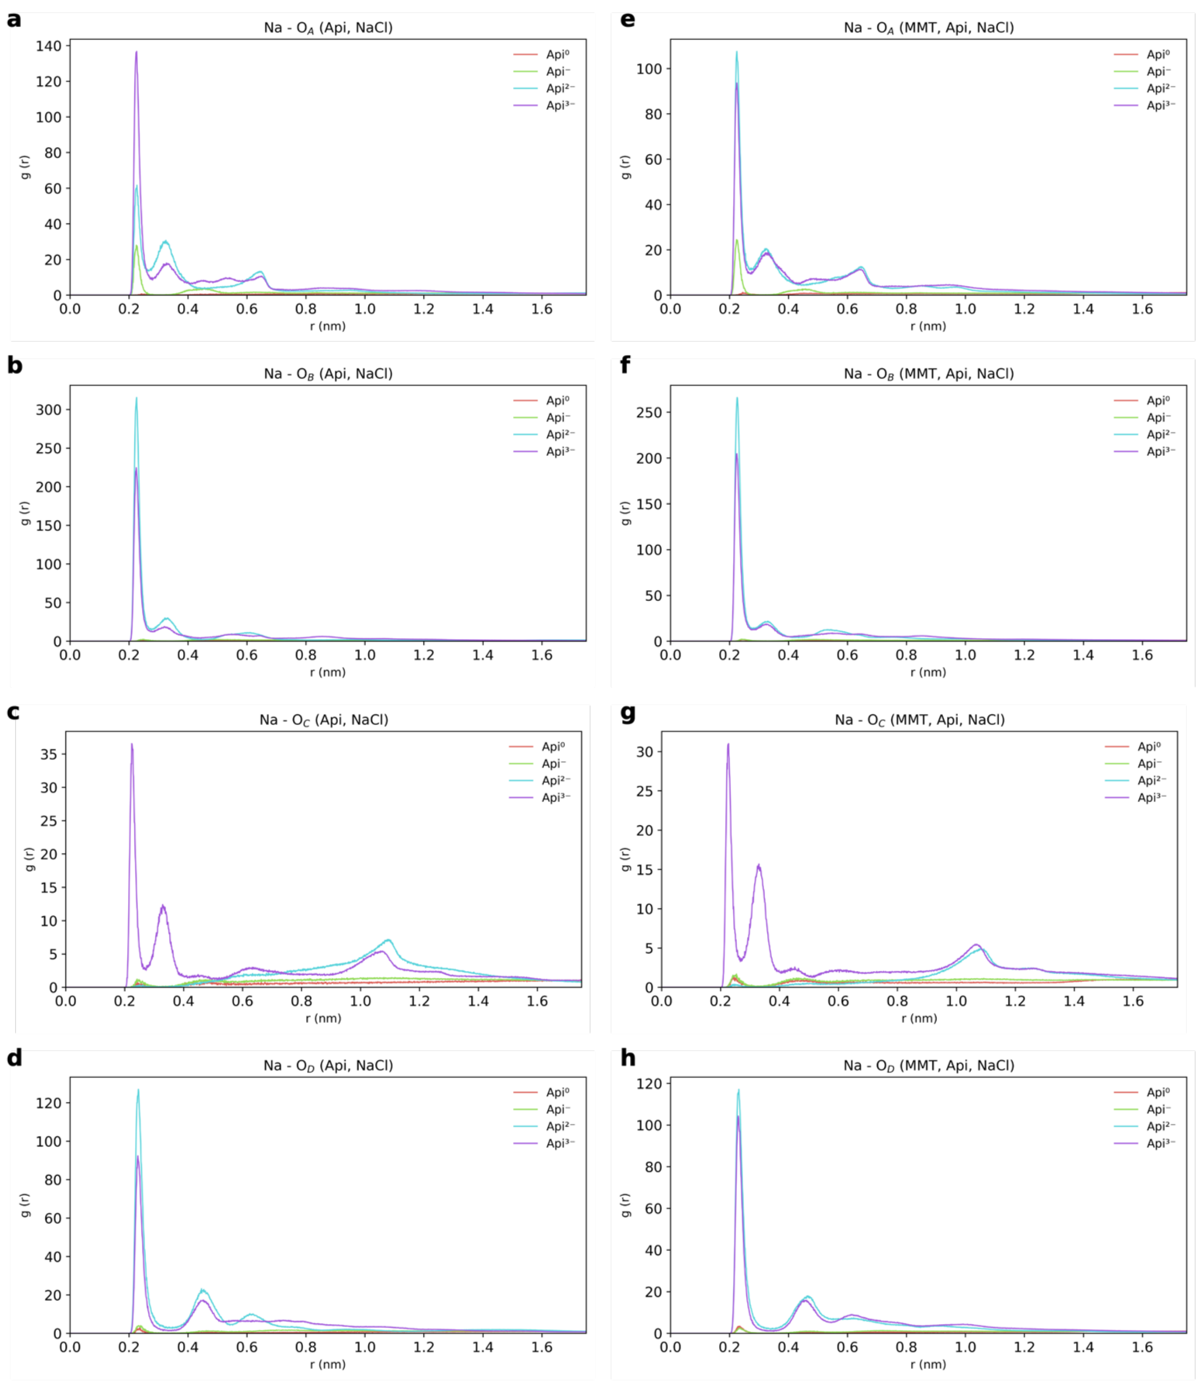


**Figure S7**: Radial distribution of O-groups on apigenin (see **Figure S1** for naming) vs $Na^+$ ion: (**a – d**) are in a 0.1M NaCl solution, (**e – f**) are in the presence of MMT and 0.1M NaCl solution.

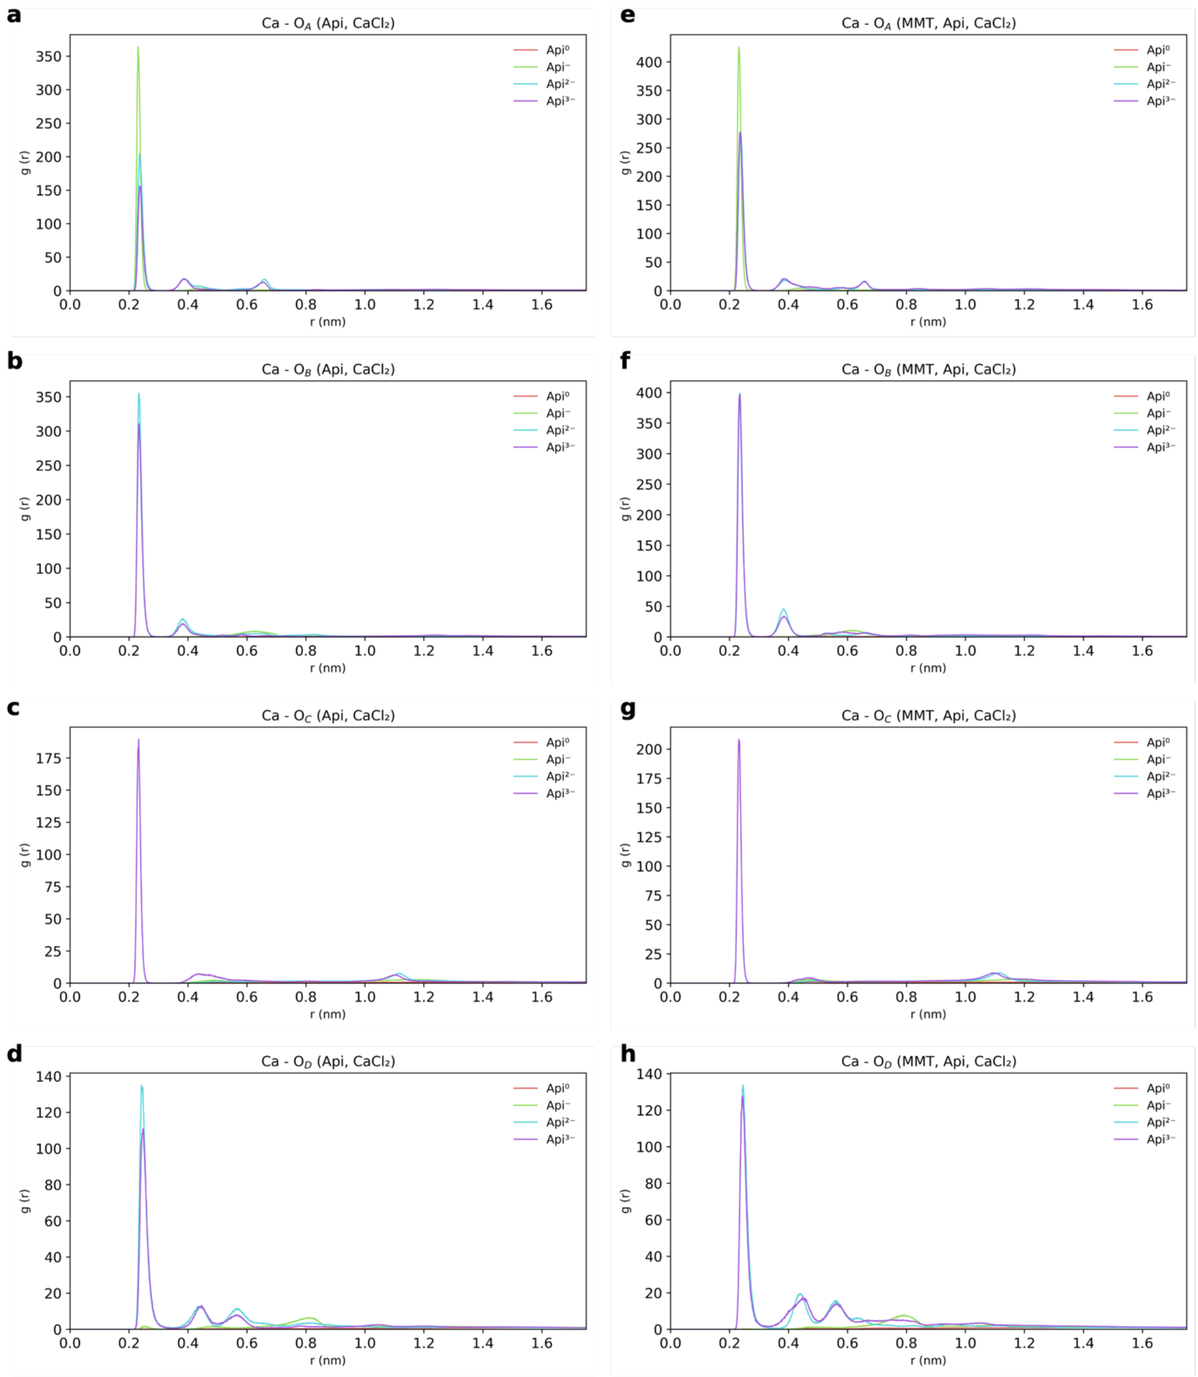


**Figure S8**: Radial distribution of O-groups on apigenin (see **Figure S1** for naming) vs $Ca^{2+}$ ion: (**a – d**) are in a 0.1M $CaCl_2$ solution, (**e – f**) are in the presence of MMT and 0.1M $CaCl_2$ solution.

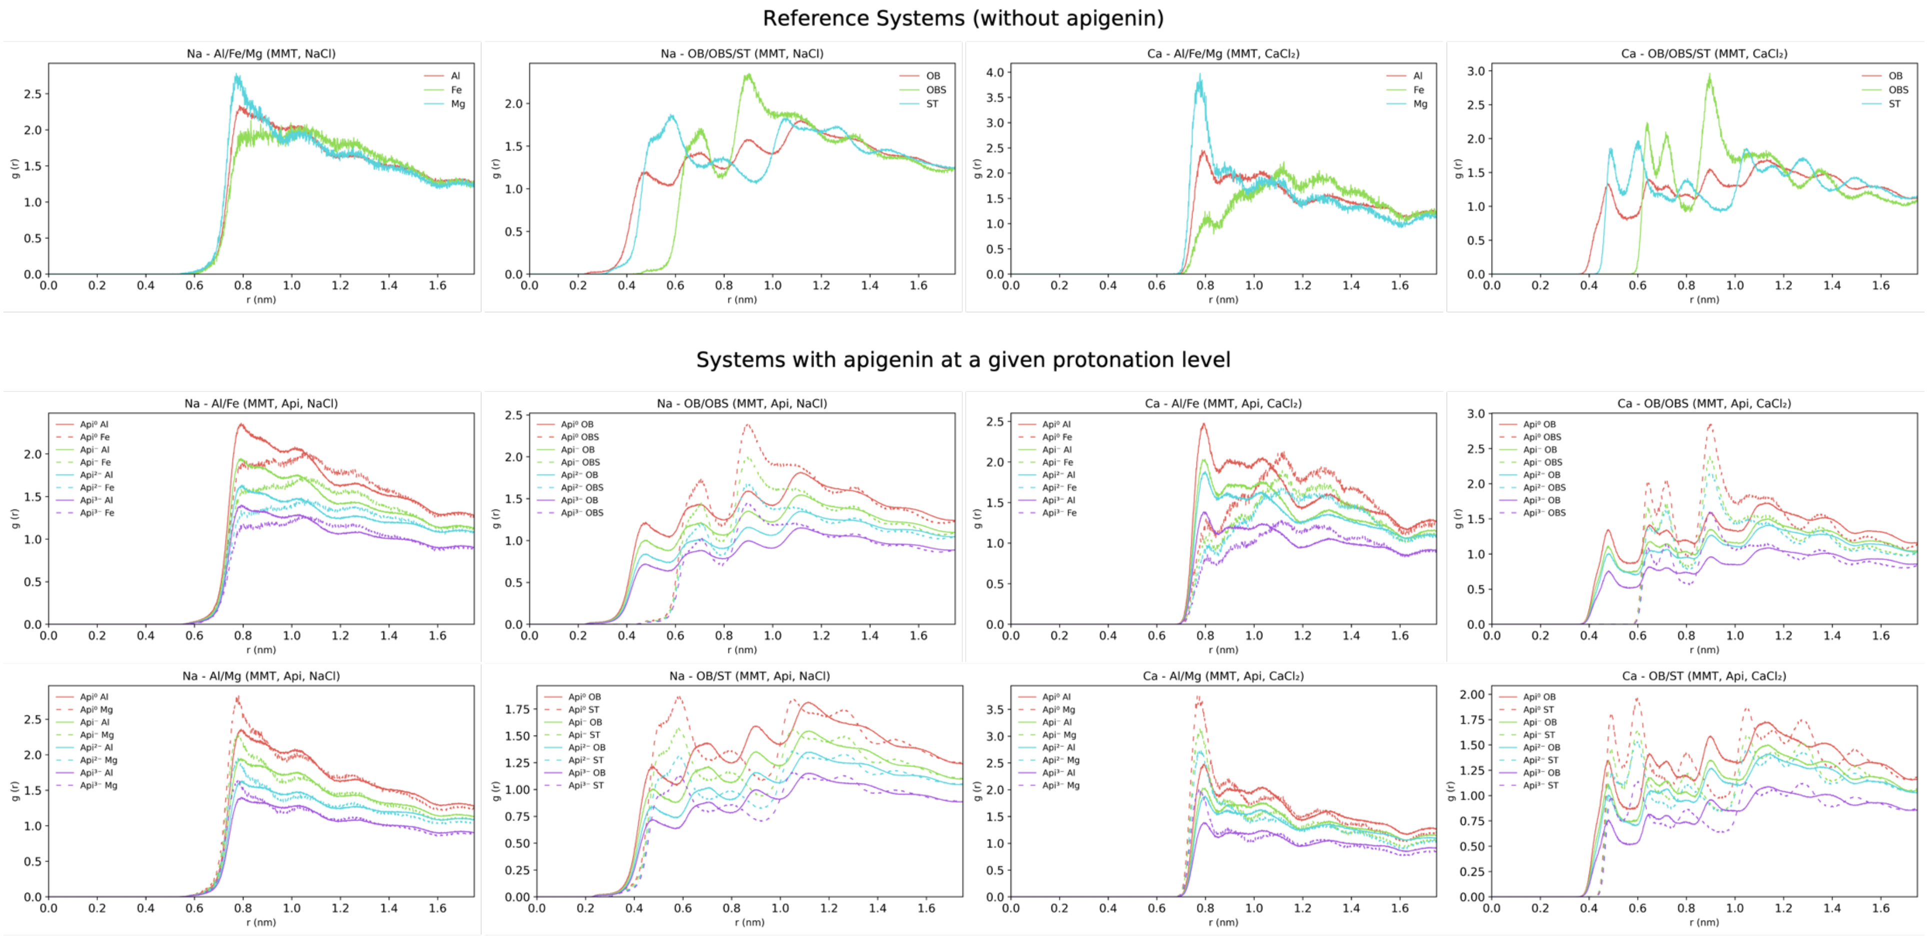


**Figure S9:** Radial distribution of clay-composing atoms vs $Na^{+}$ or $Ca^{2+}$ ions, for the reference system (top row) and apigenin-containing system. The atom names within the clay are given on the **Figure S3**
